# Supplementary material for: Non-reciprocity and multibody interactions in acoustically levitated particle systems: A three body problem
Source: arXiv:2503.12327 source file (2025-03-16)
Supplement: Supplementary file 1 [file unused_appendix.tex]

\section*{APPENDIX D: DYNAMICAL MATRIX OF THE THREE PARTICLES SYSTEM}
\begin{figure}[h!]
    \centering
    \includegraphics[width=86mm]{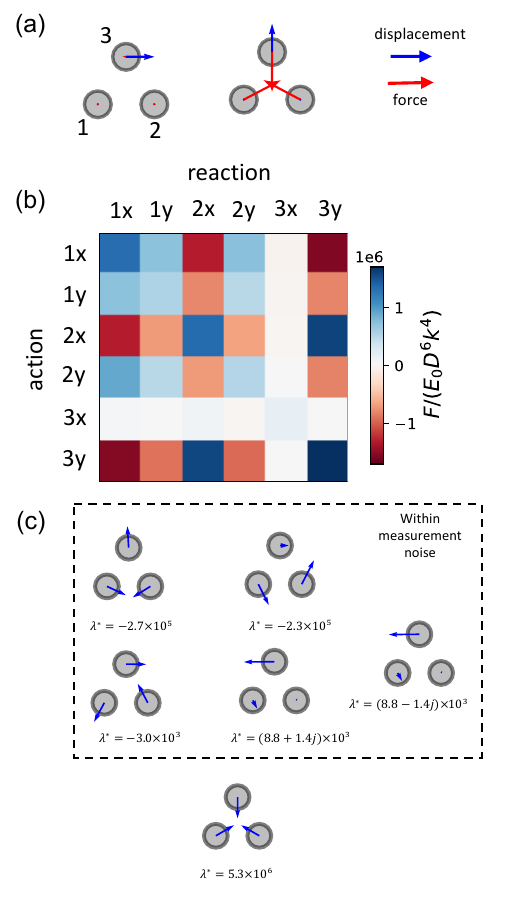}
    \caption{
    (a) the resulting forces of a displacement for particle 3 in the x (left) and y (right) directions. Blue and red arrow denotes the displacement direction and the resulting forces, respectively.
    (b) the dynamical matrix constructed by repeating the above procedure for all three particles. The row denotes the particle and direction of the displacement (action), column denotes the resulting force (reaction).
    (c) the resulting eigenmodes from the dynamical matrix. The frequency $f^*$ is specified for each mode. 
    }
    \label{fig:dyanmical_matrix}
 \end{figure}
To fully characterize the levitated three particle system, here we develop the dynamical matrix from FEM fluid simulation. 
We start by displacing particle 3 (see Fig.~\ref{fig:fig1}(c) of the main text) in the x and y direction, respectively, and obtain the resulted force on each particle, as shown in Fig.\ref{fig:dyanmical_matrix} (a). 
Notably, while the force resulting from displacing particle 3 in x direction is still restoring (opposing the direction of the displacement) it is orders of magnitude weaker than the force resulting from displacing the particle by the same amount in the y direction. 
In contrast, a linear, spring-like interaction would result in $F_{3x}=-2\cos(\pi/3)k=-k$ and $F_{3y}=-2\cos(\pi/6)k=-\sqrt{3}k$, and the restoring force in the x and y direction would be comparable.
Additionally, when particle 3 is displaced in the y direction, the forces on particles 1 and 2 are not pointing towards particle 3, which would be the case for pair-wise interactions.
As a result of the exceedingly small restoring force in the x direction, the experimentally observed three particle cluster sometimes do not always stay as equilateral triangle. 

By repeating the procedure above for each particle and displacement direction, we constructed the dynamical matrix shown in Fig.~\ref{fig:dyanmical_matrix} (b). Each element in the matrix is obtained by fitting a polynomial for $F_{ij}$ as a function of the displacement $d_i$, where $i$ and $j$ run over $1x$, $1y$, $2x$, etc..
The linear component of the polynomial fit, $k_{ij}$, gives the $D_{ij}=-k_{ij}$.

By diagonalizing the dynamical matrix, one can then obtain the eigenmodes and the corresponding frequencies, as shown in Fig.~\ref{fig:dyanmical_matrix} (c). 
The eigenvalue $\lambda^*=f^2$ here is obtained from the normalized force $F/(E_0D^6k^4)$.
The negative eigenvalue of some eigenmodes are mostly due to numerical noise.
The only eigenmode extracted accurately from the dynamic matrix is the breathing mode (bottom).


% The negative frequency could also be a result of the non-additivity of acoustic interaction.
% By construction, the dynamic matrix assumes that the interactions are additive; therefore, displacing particle 1, 2, and then 3 sequentially by the same amount should be the same as displacing all three particles together.
% In both experiment and simulation, the system preserves translational symmetry, meaning that if we globally translate the system as a rigid body, there will not be any resulting force on particles. 
% This is confirmed from FEM simulation and free drift of the trimer in experiment [Fig.~\ref{fig:dyanmical_matrix}(d), top].
% However, as the dynamic matrix is obtained from displacing one particle while keeping all other particles fixed, the resulting force from rigid body translation is non-zero (bottom).
% This demonstrates that for non-pairwise additive interactions, one has to be cautious using dynamic matrix methodology. 
% In fact, this is exact the reason that we do not recover the two translational modes in x and y directions in Fig.~\ref{fig:dyanmical_matrix}(c).

 \section*{APPENDIX F: THRUST MAGNITUDE OF SELF-PROPULSION}
% \subsection*{Thrust magnitude of self-propulsion}
\begin{figure}[h]
    \centering
    \includegraphics[width=3in]{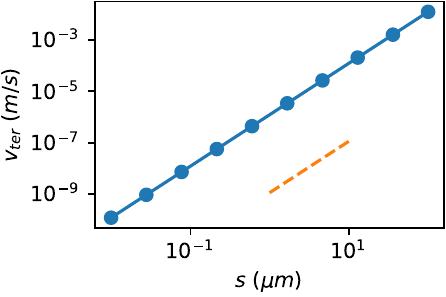}
    \caption{The terminal velocity $v_{ter}$ in the +y direction for the self-propulsion state as a function of the acoustic oscillation amplitude of the driving $s$, as obtained from FEM fluid simulation. Orange dashed line represents $\sum_i F^i_y \propto s^2$ scaling.
    }
    \label{fig:limit_energy_fraction}
 \end{figure}

Experimentally, it is challenging to measure the self-propulsion speed as a function of the energy density $E_0$ because of the presence of the confining force in the xy plane. 
Nevertheless, we can perform FEM fluid simulation to extract the scaling relationship between the self-propulsion velocity and driving amplitude $s$ for the dimer-and-particle configuration shown in Fig.~\ref{fig:fig1}(g) of the main text.
The total force on all particles in the +y direction scales as $\sum_i F^i_y \propto s^2$, which is expected as $F^i_y\propto E_0\propto s^2$.
Under Stokes' drag, the terminal velocity will be $v_{ter}=\sum_i F^i_y/\gamma\propto s^2$, where $\gamma=6\pi\mu (D/2+\delta_{\nu})$ is the Stokes' drag on a single particle, $\mu$ is the dynamic viscosity of air, and $\delta_{\nu}\approx 12\mu m$ is the size of the viscous boundary layer.

This result is consistent with the theory results from Nadal et.~al. \cite{nadal_asymmetric_2014}. 
However, as also explained in the main text, more recent theoretical results show that `no net motion can arise at $O(\epsilon Re)$ from a time reciprocal oscillation' \cite{lippera_no_2019}, where $\epsilon$ is an asphericity parameter, and those authors argue that self-propulsion can only arise from higher order terms in $O(\epsilon Re)$.
If self-propulsion arises from higher order terms in $O(\epsilon Re)$, the magnitude of the force will scale faster than $s^2$, contradicting with our result above.

Additionally, recent theoretic studies suggest that density difference and hence rotational oscillations of the particles are required for self-propulsion\cite{collis_autonomous_2017,nadal_acoustic_2020}.
However, we do observe rotational oscillations experimentally; all particles are made of the same material, and density difference should be negligible.
In FEM fluid simulation, we also assume identical particle densities and do not allow rotational motion of the particles.
We therefore believe that time-reciprocal oscillation can naturally give rise to self-propulsion of an asymmetric particle; this can be entirely a result of the shape asymmetry, and assumptions about the density of the particle or oscillation motion are not required.
There is therefore a gap between the current theory development and the experimental observations, and more work from theory, numerical simulations, and experiments are needed to close the gap.

 \section*{APPENDIX G: KINETIC ENERGY OF EACH PARTICLE IN LIMIT CYCLES}
\begin{figure}[h]
    \centering
    \includegraphics[width=3in]{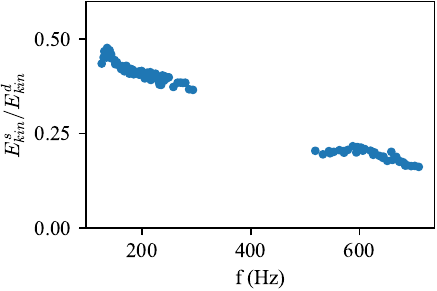}
    \caption{The ratio of the time-averaged kinetic energy between the single particle and the dimer particles, $E_{kin}^s/E_{kin}^d$, as a function of oscillation frequency.
    }
    \label{fig:limit_energy_fraction}
 \end{figure}
To further show the difference between regime I and II limit cycles, we calculate the time-averaged kinetic energy of the single particle, $E_{kin}^s$, and the dimer particles, $E_{kin}^d$. 
$E_{kin}^s/E_{kin}^d$ as a function of oscillation frequency is shown in Fig.~\ref{fig:limit_energy_fraction}.
For regime I, while the ratio slightly decreases with increasing oscillation frequency, the values are within the range of 0.35-0.5, meaning that the single particle oscillate as much as one of the dimer particles. 
In contrast, $E_{kin}^s/E_{kin}^d\approx 0.15$ in regime II.
The single particle therefore oscillates slower at regime II.
